# Supplementary material for: Multi-band Weighted $l_p$ Norm Minimization for Image Denoising
Source: arXiv:1901.04206 source file (2020-06-23)
Supplement: Supplementary file 1 [file supplement.pdf]

# Supplementary Materials to "Multi-band Weighted $l_p$ Norm Minimization for Color Image and Multispectral Image Denoising"

## 1 Proof of Theorems

**Theroem 2**. Problem (6) is equivalent to problem (9), that they share the same solution.

*Proof.* According to Theorem 1, we have

$$\begin{aligned} W, X \in M_{m,n} \quad &\Rightarrow \quad \sigma_i(WX) \le \sigma_i(W)\, \|X\| \\ &for\ 1 \le i \le \min(m,n). \end{aligned} \tag{1}$$

Since the singular values and the spectral norm do not change under transposition, it follows

$$\sigma_i(WX) \le \|W\|\, \sigma_i(X) \tag{2}$$

as well. Hence, we have

$$\begin{aligned} \|X\|_{\omega,S_p}^p =& \sum\nolimits_{i=1}^{\min\{m,n\}} \omega_i \sigma_i^p(X) \\ \ge& \|W\|^{-1} \sum\nolimits_{i=1}^{\min\{m,n\}} \omega_i \sigma_i^p(WX) \\ =& \|W\|^{-1} \|WX\|_{\omega,S_p}^p . \end{aligned} \tag{3}$$

Since $W$ is calculated from the image, it can be considered as a constant. Then,

$$\|W(X-Y)\|_F^2 + \|X\|_{\omega,S_p}^p \ge \|W(X-Y)\|_F^2 + \lambda \|WX\|_{\omega,S_p}^p \tag{4}$$

where $\lambda = \|W\|^{-1}$, $\lambda$ is a constant. □

**Theroem 4**. *Let the SVD of $WY \in R^{m\times n}$ be $WY = U\Delta V^T$ with $\Delta = diag(\delta_1, ...\delta_r), r = \min\{m,n\}$. Then an optimal solution to (9) is $X = W^{-1}U\Sigma V^T$ with $\Sigma = diag(\sigma_1, ...\sigma_r)$, where $\sigma_i$ is given by solving the problem below:*

$$\begin{aligned} &\min_{\sigma_1,...\sigma_r} \sum_{i=1}^{r} \left[ (\sigma_i - \delta_i)^2 + \lambda w_i \sigma_i^p \right],\ i = 1, \dots r \\ &s.t.\ \sigma_i \ge 0,\ and\ \sigma_i \ge \sigma_j,\ for\ i \le j \end{aligned} \tag{5}$$

*Proof.* Suppose the SVD of $WX$ and $WY$ are $WX = Q\Sigma R^T$ and $WY = U\Delta V^T$, where $\Sigma$ and $\Delta$ are the diagonal matrix with the non-ascending order. By using Neuman's trace inequality in Theorem 3, we have

$$\begin{aligned} \|WX - WY\|_F^2 =& tr(\Sigma^T\Sigma) + tr(\Delta^T\Delta) - 2tr((WX)^T WY) \\ \ge& tr(\Sigma^T\Sigma) + tr(\Delta^T\Delta) - 2tr(\Sigma^T\Delta) \\ =& \|\Sigma - \Delta\|_F^2 , \end{aligned} \tag{6}$$

where the equality holds if and only if $Q = U$ and $R = V$. This means that

$$\|W(X-Y)\|_F^2 + \lambda \|WX\|_{\omega,S_p}^p \geq \|\Sigma - \Delta\|_F^2 + \lambda \|WX\|_{\omega,S_p}^p$$
$$= \min_{\sigma_1,\dots\sigma_r} \sum_{i=1}^{r} \Big[(\sigma_i - \delta_i)^2 + \lambda w_i \sigma_i^p\Big]. \tag{7}$$

This completes the proof of Theorem 4. □

## 2 Detailed Description of Datasets and More Results on the CAVE

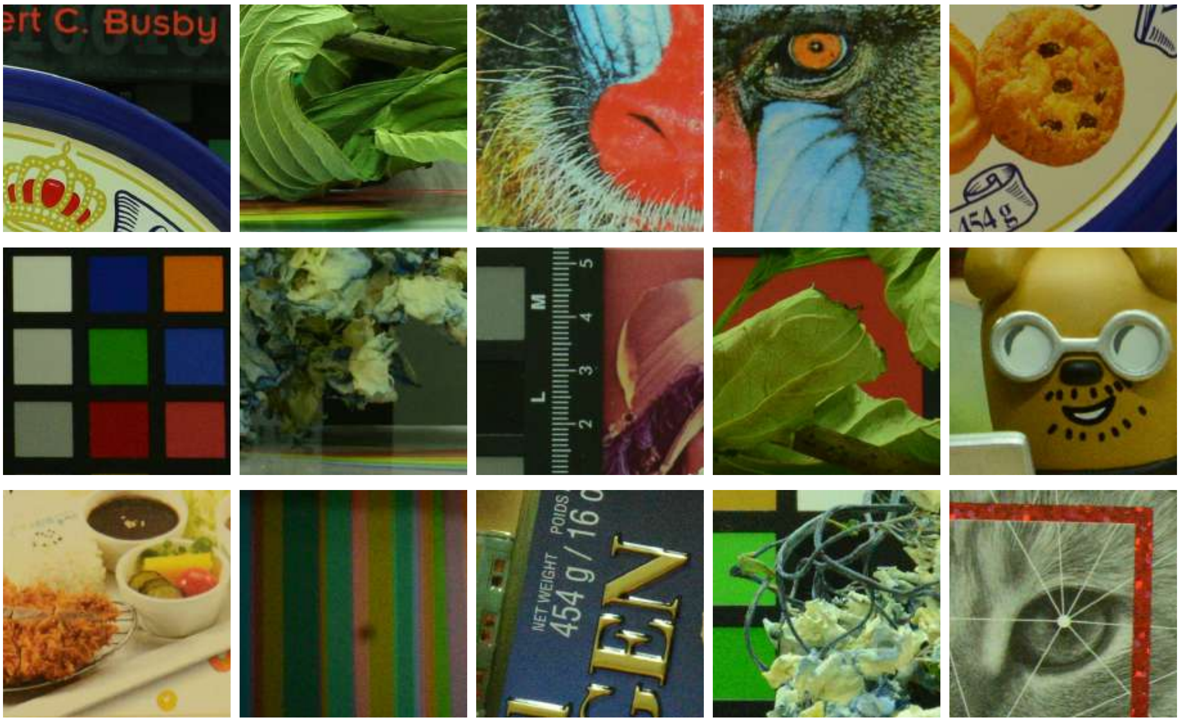


Figure 1: The 15 cropped real noisy images.

Table 1: The detailed information of the cropped regions from the dataset[Xu et al., 2018, Abdelhamed et al., 2018].

| Name | of Images | of Scenes | Original Size | Cropped Size | Brand | ISO |
|---|---|---|---|---|---|---|
| Dataset 2 | 100 | 40 | $3000 \times 3000$ | $512 \times 512$ | Canon 5D Mark II<br>Canon 80D,600D<br>Nikon D800,Sony A7 II | 0.8k,1.6k<br>1.8k,3.2k<br>5k,6.4k,12.8k |
| Dataset 3 | 150 | 10 | About<br>$4000 \times 3000$<br>$5000 \times 3000$ | $512 \times 512$ | iPhone 7, LG G4<br>Google Pixel, Nexus 6<br>Galaxy S6 Edge | 15 different<br>ISO levels<br>(50-10000) |

Table 2: Different simulated results of different methods on CAVE dataset.

| | Index | BM4D | LRTA | SDS | ANLM | NMF | BM3D | LRMR | ISTReg | LLRT | MBWPNM |
|---|---|---|---|---|---|---|---|---|---|---|---|
| 1 | PSNR | 36.64 | 30.74 | 31.55 | 38.39 | 35.51 | 34.54 | 33.95 | 41.94 | 42.53 | **42.66** |
| | SSIM | 0.8998 | 0.6926 | 0.8354 | 0.9103 | 0.9069 | 0.8730 | 0.7976 | 0.9498 | 0.9712 | **0.9714** |
| | ERGAS | 84.08 | 177.29 | 177.42 | 74.11 | 95.43 | 102.21 | 122.98 | 49.38 | **43.56** | 43.90 |
| | SAM | 0.3928 | 0.6013 | 0.5244 | 0.3223 | 0.3121 | 0.3491 | 0.5404 | 0.3026 | **0.1364** | 0.1466 |
| 2 | PSNR | 31.70 | 25.21 | 23.67 | 33.38 | 29.12 | 28.68 | 28.41 | 38.12 | 37.62 | **39.08** |
| | SSIM | 0.8067 | 0.4924 | 0.6291 | 0.7777 | 0.8338 | 0.7747 | 0.5658 | 0.8958 | 0.9336 | **0.9467** |
| | ERGAS | 149.78 | 338.03 | 407.82 | 133.26 | 193.77 | 199.62 | 233.65 | 75.17 | 73.97 | **65.58** |
| | SAM | 0.5645 | 0.7907 | 0.8088 | 0.4811 | 0.4710 | 0.5066 | 0.7309 | 0.4549 | 0.2155 | **0.2085** |
| 3 | PSNR | 28.63 | 21.96 | 19.36 | 30.20 | 25.68 | 28.11 | 25.22 | 36.10 | 36.10 | **37.18** |
| | SSIM | 0.7389 | 0.3837 | 0.4686 | 0.6627 | 0.7793 | 0.7530 | 0.4015 | 0.8678 | 0.9198 | **0.9272** |
| | ERGAS | 214.49 | 492.86 | 651.08 | 193.05 | 287.55 | 211.19 | 339.68 | 94.28 | 88.59 | **81.56** |
| | SAM | 0.6747 | 0.8962 | 0.9582 | 0.5910 | 0.5620 | 0.5142 | 0.8324 | 0.4883 | **0.2351** | 0.2444 |
| 4 | PSNR | 26.39 | 19.59 | 16.60 | 27.89 | 23.27 | 26.38 | 22.99 | 33.09 | 35.01 | **35.52** |
| | SSIM | 0.6869 | 0.3125 | 0.3750 | 0.5754 | 0.7376 | 0.7132 | 0.2929 | 0.8424 | **0.9062** | 0.9046 |
| | ERGAS | 278.44 | 648.86 | 884.87 | 252.48 | 380.47 | 258.15 | 442.02 | 136.10 | 101.03 | **98.21** |
| | SAM | 0.7534 | 0.9706 | 1.0434 | 0.6715 | 0.6259 | 0.5684 | 0.9031 | 0.5036 | **0.2536** | 0.2856 |

# 3 More Visual comparisons on the Kodak PhotoCD Dataset

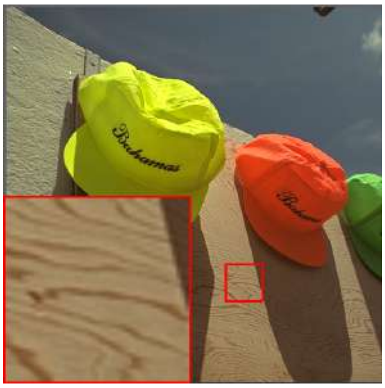

(a) Ground Truth

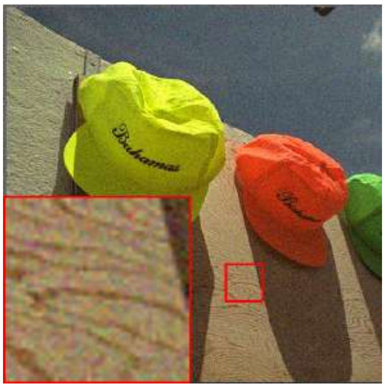

(b) Noisy Image,PSNR=22.30dB

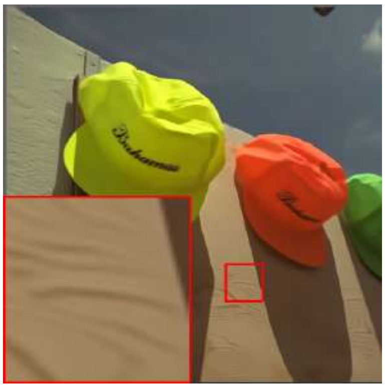

(c) CBM3D, PSNR=32.52dB

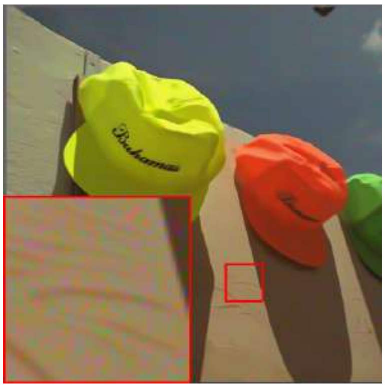

(d) NCSR, PSNR=33.45dB

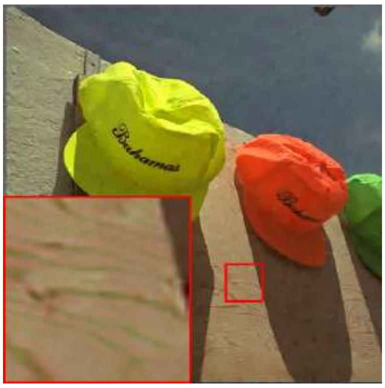

(e) EPLL, PSNR=34.08dB

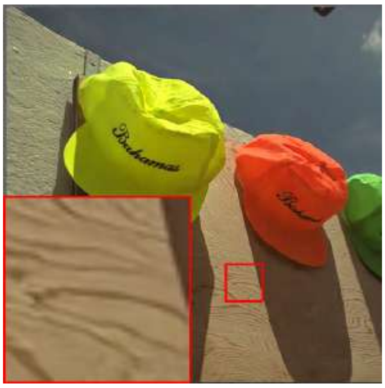

(f) DnCNN, PSNR=35.83dB

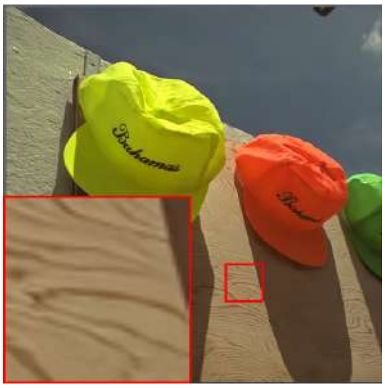

(g) FFDNet, PSNR=36.28dB

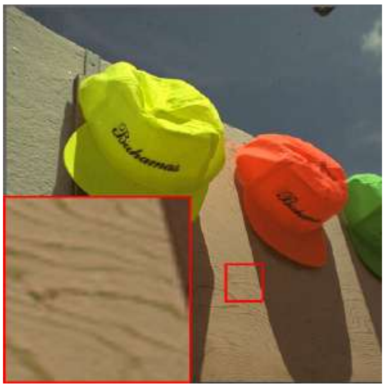

(h) MCWNNM, PSNR=35.79dB

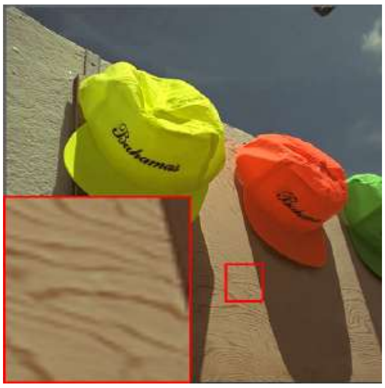

(i) MBWPNM, PSNR=36.40dB

Figure 2: Denoised images of different methods on the image "kodim03" degraded by AWGN with different standard deviations of $\sigma_r$=5,$\sigma_g$=30,$\sigma_b$=15 on R, G, B channels, respectively. The images are better to be zoomed in on screen.

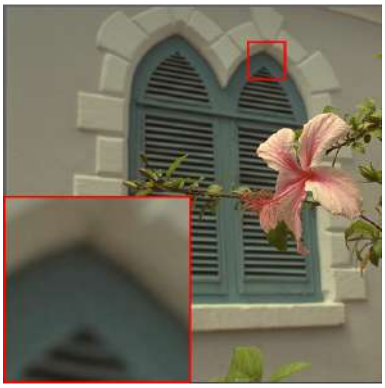

(a) Ground Truth

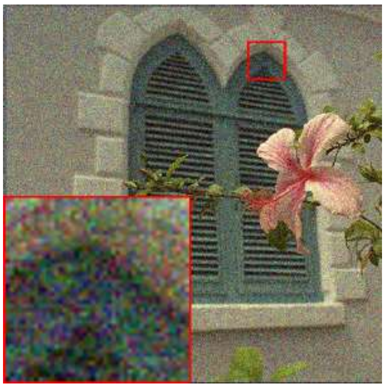

(b) Noisy Image,PSNR=21.00dB

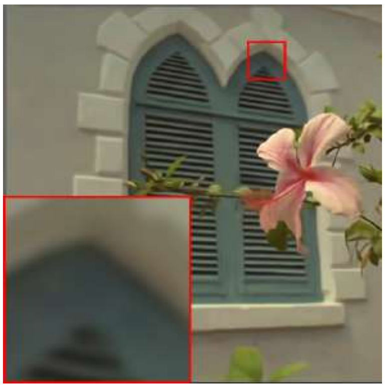

(c) CBM3D, PSNR=31.31dB

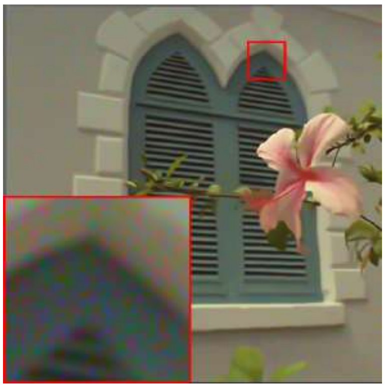

(d) NCSR, PSNR=32.19dB

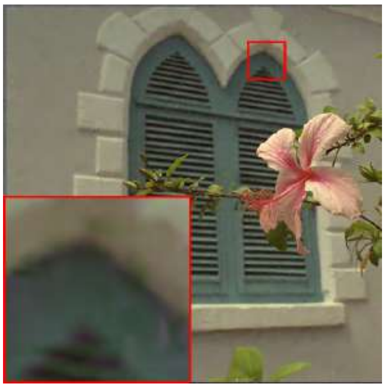

(e) EPLL, PSNR=32.34dB

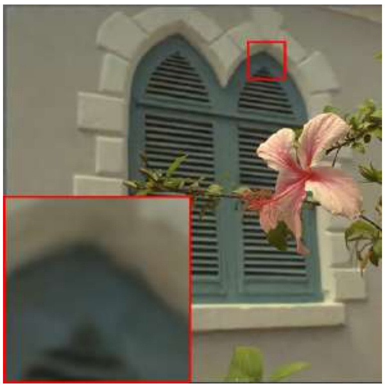

(f) DnCNN, PSNR=34.43dB

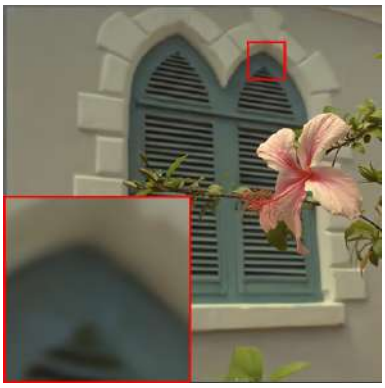

(g) FFDNet, PSNR=34.54dB

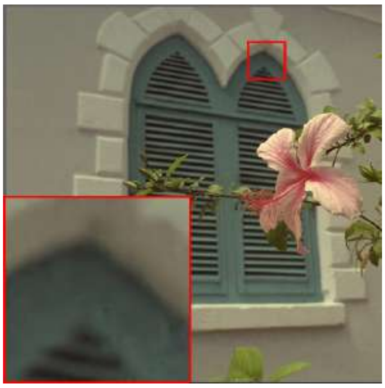

(h) MCWNNM, PSNR=33.83dB

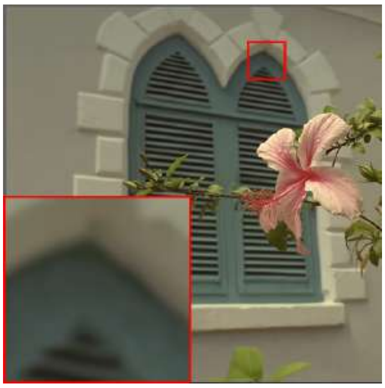

(i) MBWPNM, PSNR=34.88dB

Figure 3: Denoised images of different methods on the image "kodim03" degraded by AWGN with different standard deviations of $\sigma_r$=25,$\sigma_g$=5,$\sigma_b$=30 on R, G, B channels, respectively. The images are better to be zoomed in on screen.

# 4 More Visual comparisons on [Nam et al., 2016]

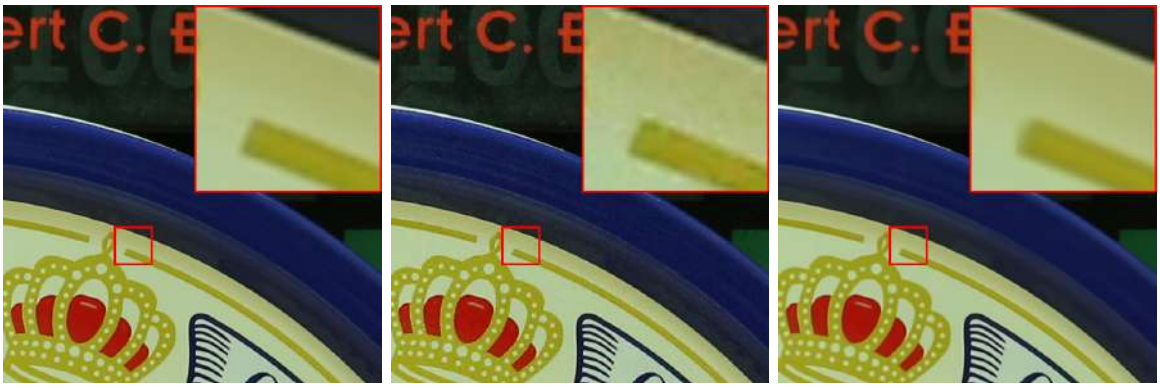

(a) Ground Truth (b) Noisy Image, PSNR=37.00dB (c) CBM3D, PSNR=38.25dB

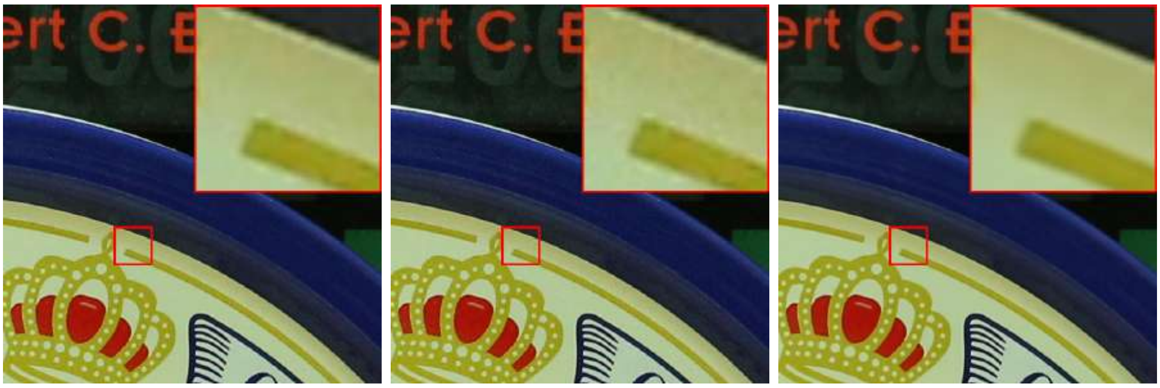

(d) NCSR, PSNR=38.02dB (e) EPLL, PSNR=37.00dB (f) Guided, PSNR=40.82dB

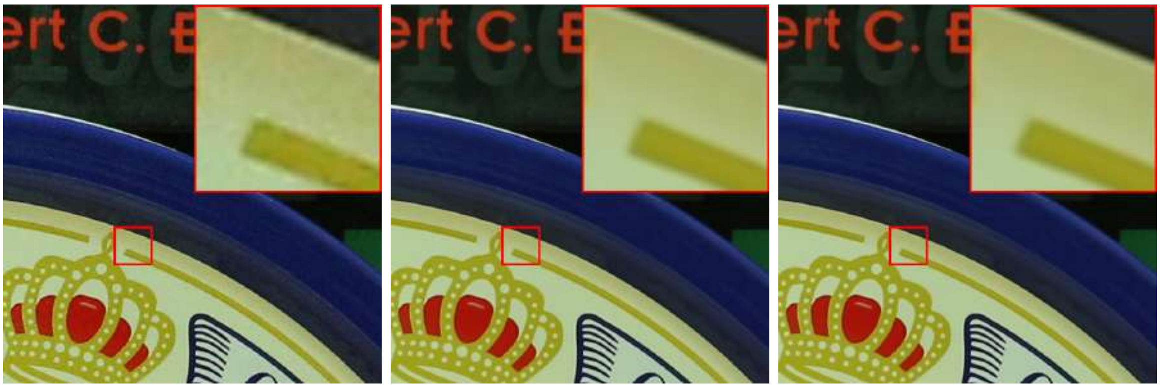

(g) FFDNet, PSNR=37.05dB (h) MCWNNM, PSNR=41.20dB (i) MBWPNM, PSNR=41.21dB

Figure 4: Denoised images of a region cropped from the real noisy image "Canon 5D Mark 3 ISO=3200 1" by different methods. The estimated noise levels of R, G, and B channels are 1.58, 1.57, and 1.61, respectively.The images are better to be zoomed in on screen.

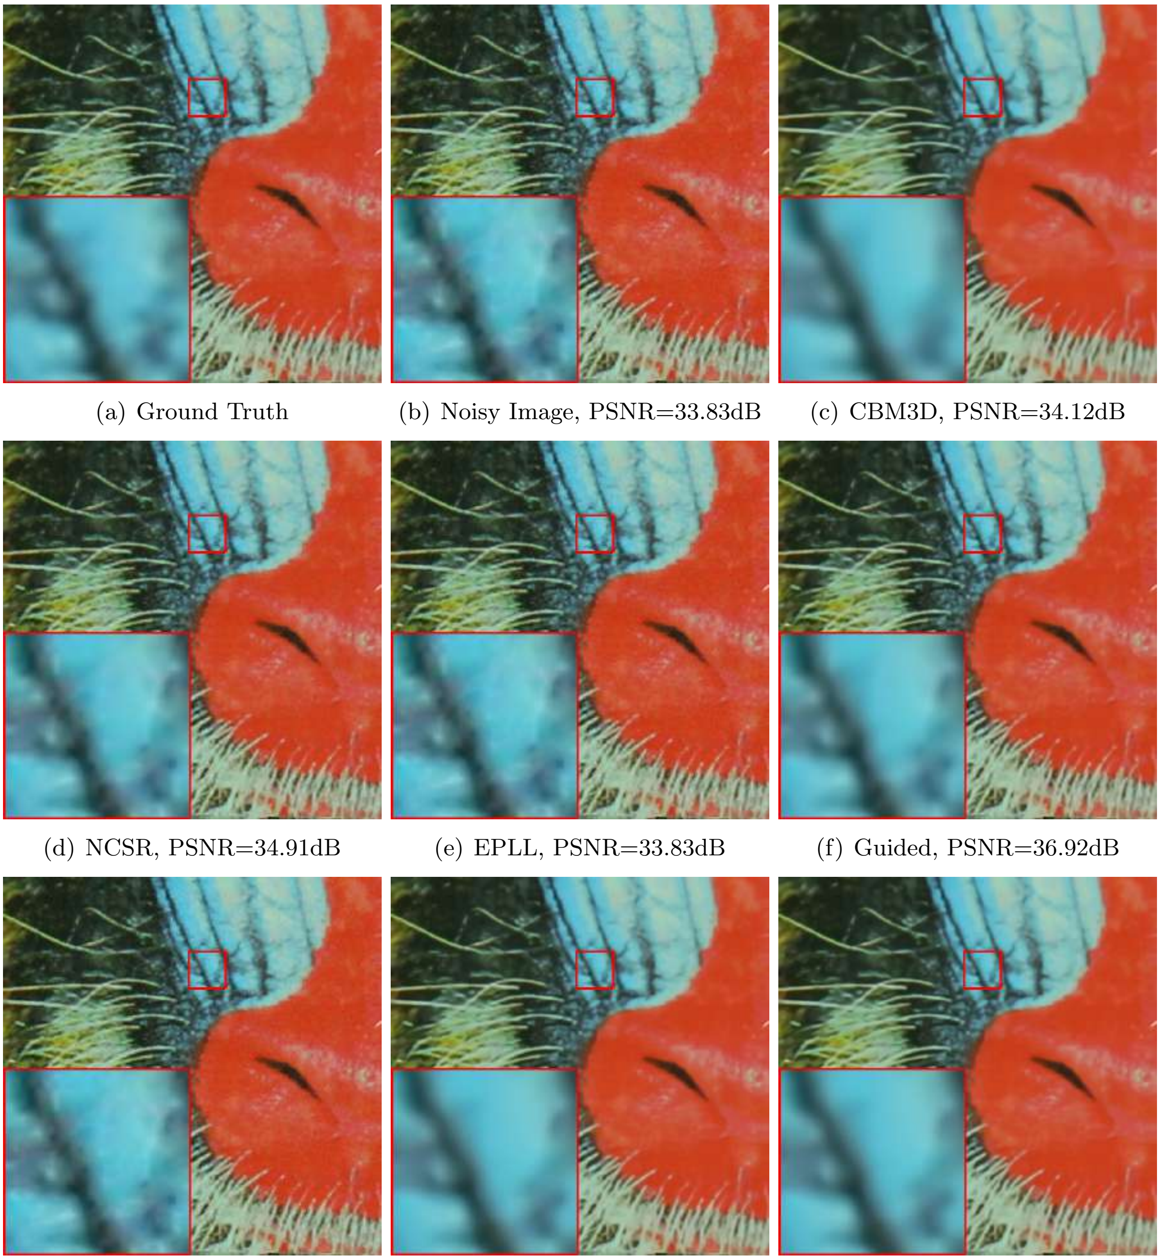

(a) Ground Truth (b) Noisy Image, PSNR=33.83dB (c) CBM3D, PSNR=34.12dB

(d) NCSR, PSNR=34.91dB (e) EPLL, PSNR=33.83dB (f) Guided, PSNR=36.92dB

(g) FFDNet, PSNR=33.86dB (h) MCWNNM, PSNR=36.48dB (i) MBWPNM, PSNR=37.14dB

Figure 5: Denoised images of a region cropped from the real noisy image "Canon 5D Mark 3 ISO=3200 3" by different methods. The estimated noise levels of R, G, and B channels are 2.41, 2.38, and 2.44, respectively.The images are better to be zoomed in on screen.

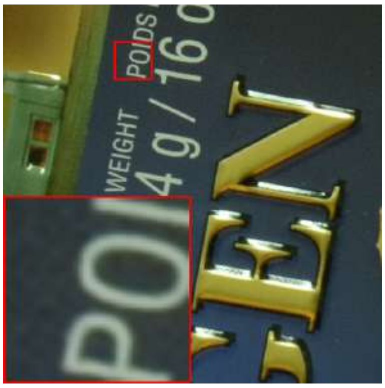


(a) Ground Truth

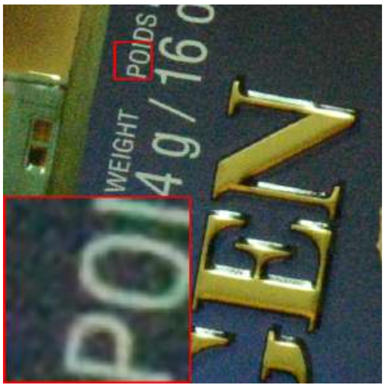


(b) Noisy Image, PSNR=29.63dB

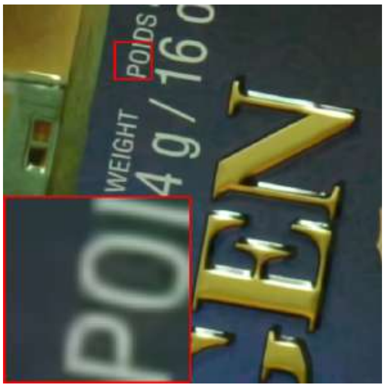


(c) CBM3D, PSNR=34.63dB

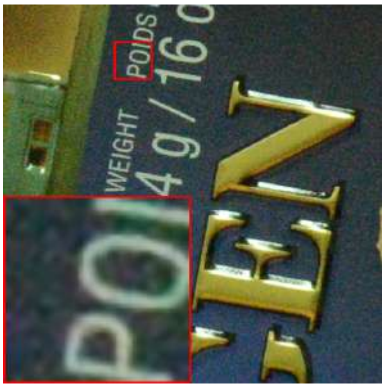


(d) NCSR, PSNR=30.09dB

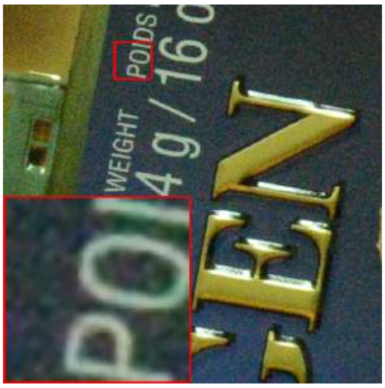


(e) EPLL, PSNR=29.63dB

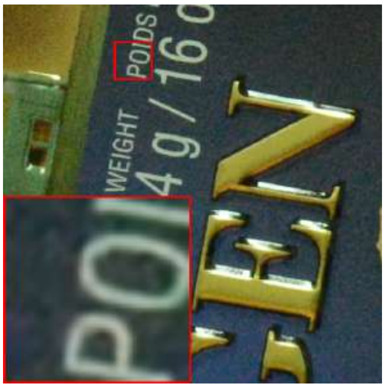


(f) Guided, PSNR=33.01dB

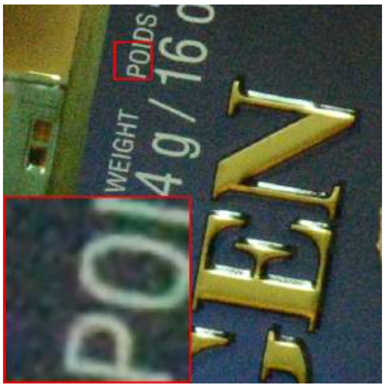


(g) FFDNet, PSNR=29.65dB

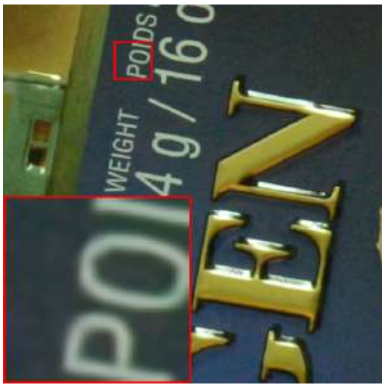


(h) MCWNNM, PSNR=34.85dB

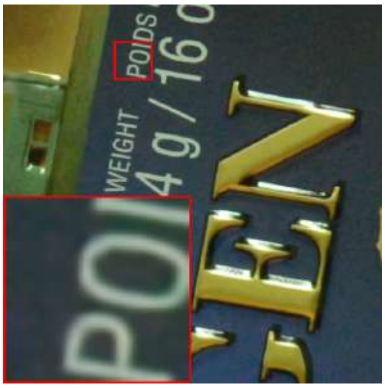


(i) MBWPNM, PSNR=34.92dB

Figure 6: Denoised images of a region cropped from the real noisy image "Nikon D800 ISO=6400 1" by different methods. The estimated noise levels of R, G, and B channels are 2.43, 2.36, and 2.05, respectively. The images are better to be zoomed in on screen.

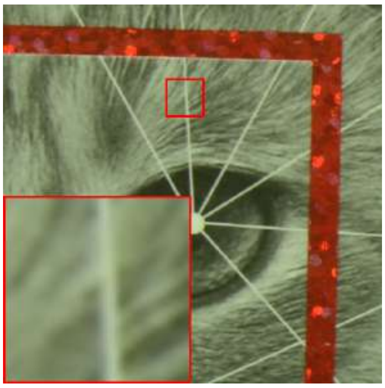

(a) Ground Truth

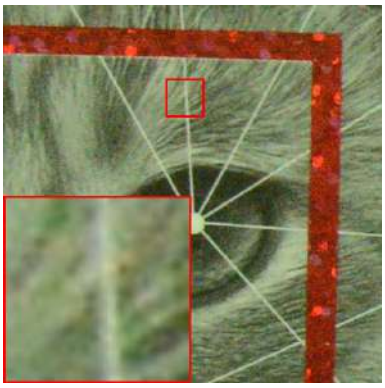

(b) Noisy Image, PSNR=29.87dB

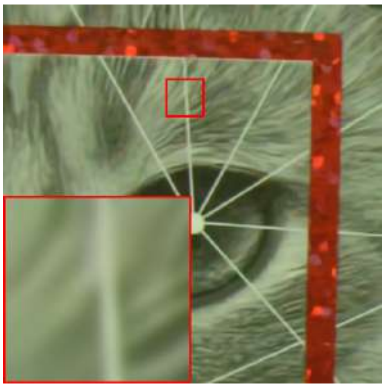

(c) CBM3D, PSNR=33.61dB

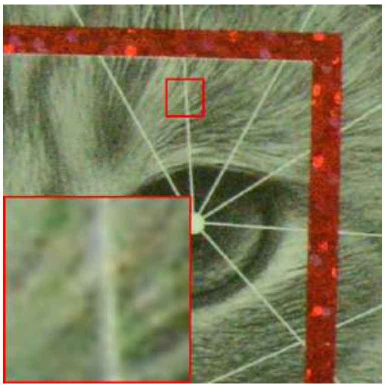

(d) NCSR, PSNR=30.12dB

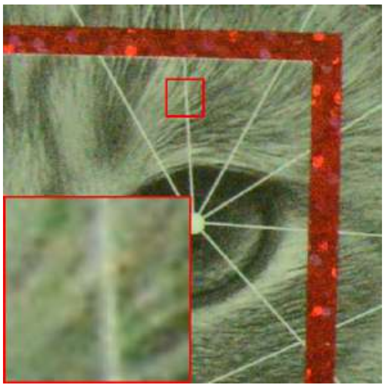

(e) EPLL, PSNR=29.87dB

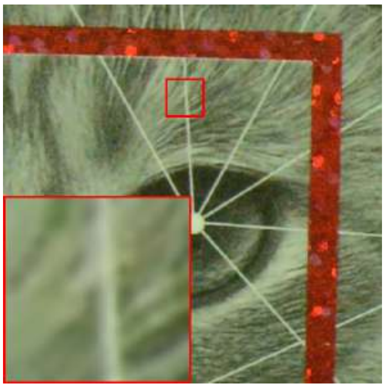

(f) Guided, PSNR=32.96dB

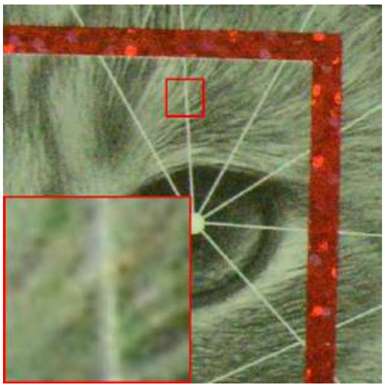

(g) FFDNet, PSNR=29.88dB

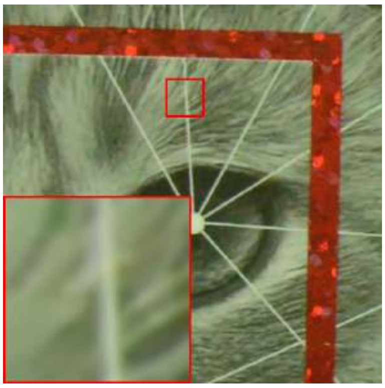

(h) MCWNNM, PSNR=33.97dB

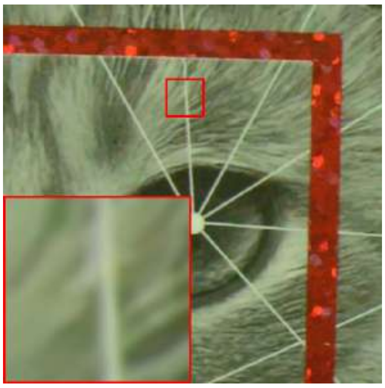

(i) MBWPNM, PSNR=34.09dB

Figure 7: Denoised images of a region cropped from the real noisy image "Nikon D800 ISO=6400 3" by different methods. The estimated noise levels of R, G, and B channels are 1.71, 1.64, and 1.79, respectively. The images are better to be zoomed in on screen.

# References

Abdelrahman Abdelhamed, Stephen Lin, and Michael S Brown. A high-quality denoising dataset for smartphone cameras. In *Proceedings of the IEEE Conference on Computer Vision and Pattern Recognition*, pages 1692–1700, 2018.

Seonghyeon Nam, Youngbae Hwang, Yasuyuki Matsushita, and Seon Joo Kim. A holistic approach to cross-channel image noise modeling and its application to image denoising. In *Proceedings of the IEEE Conference on Computer Vision and Pattern Recognition*, pages 1683–1691, 2016.

Jun Xu, Hui Li, Zhetong Liang, David Zhang, and Lei Zhang. Real-world noisy image denoising: A new benchmark. *arXiv preprint arXiv:1804.02603*, 2018.
